# Supplementary material for: Unified Unsupervised Anomaly Detection via Matching Cost Filtering
Source: arXiv:2510.03363 source file (2025-10-08)

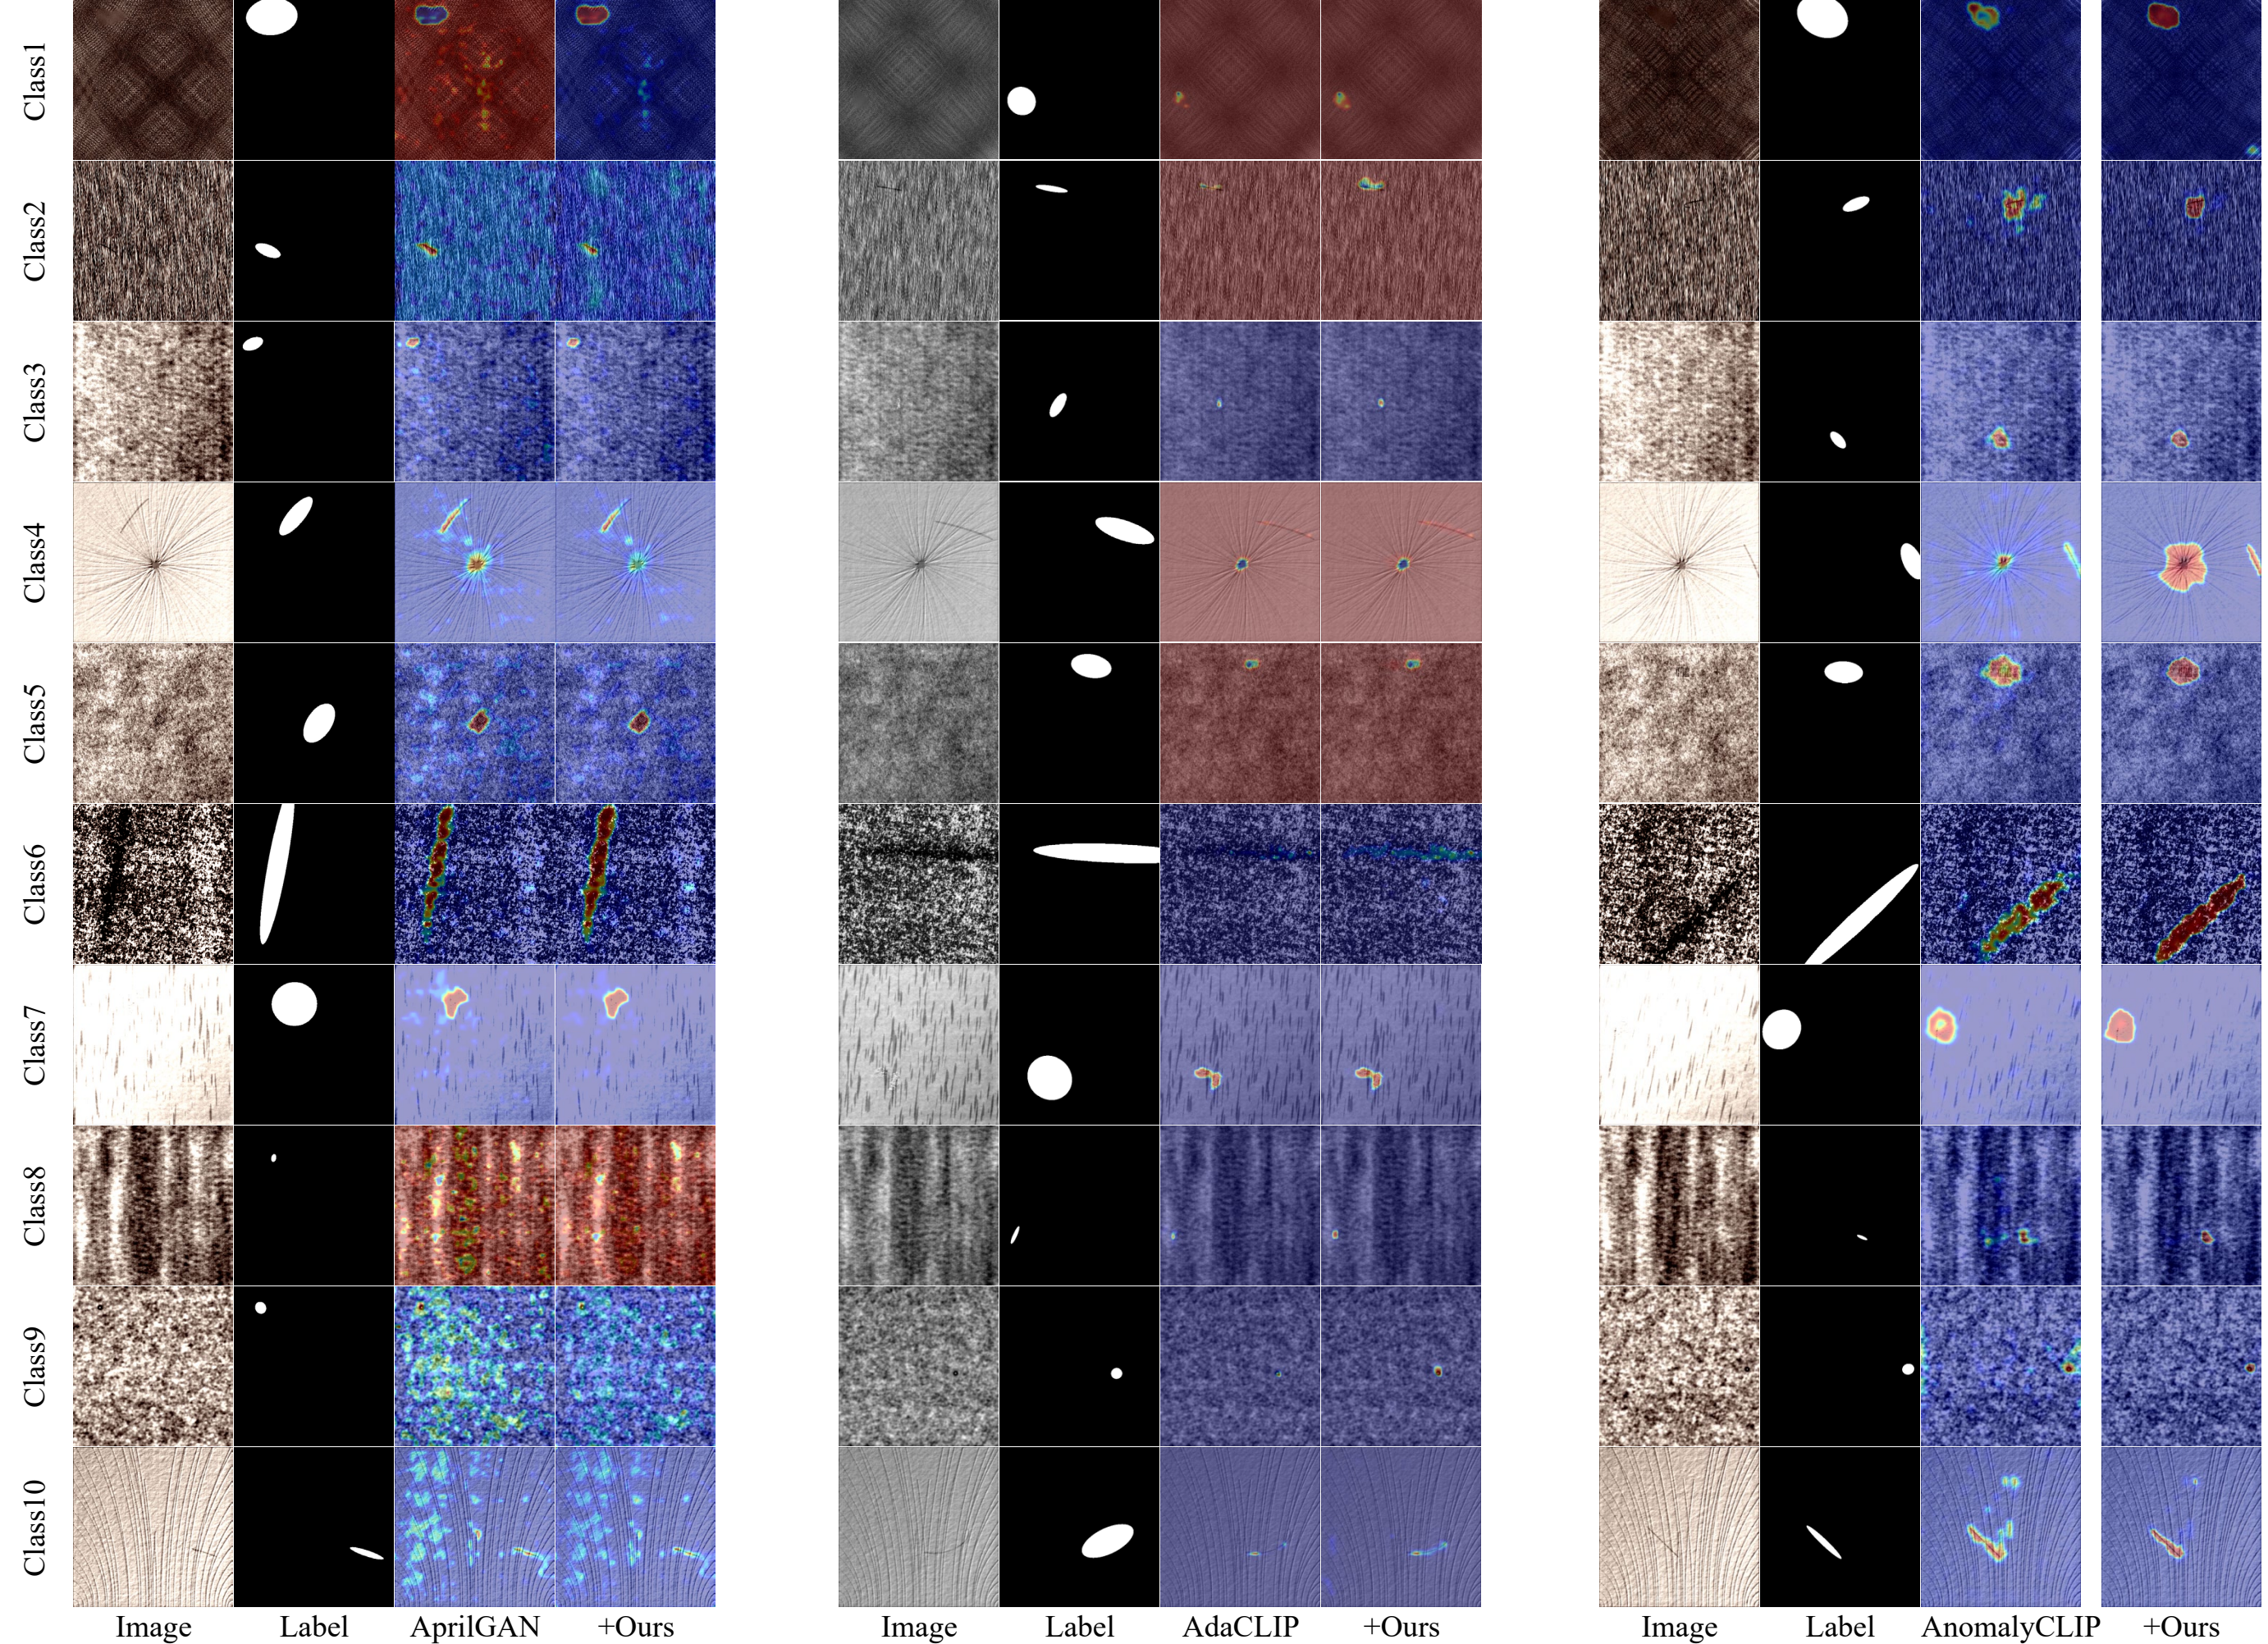

Supplement: Supplementary file 1 [file appendix_DAGM.pdf]
